# Supplementary material for: MyStyle++: A Controllable Personalized Generative Prior
Source: arXiv:2306.04865 source file (2023-10-10)
Supplement: Supplementary file 1 [file appendix.tex]

\section{Suppementary Materials}

% ----------------------------------------------------------------------------
% ----------------------------------------------------------------------------
% ----------------------------------------------------------------------------

In this supplementary materials, we offer additional visual and numerical comparisons against MyStyle\_P and MyStyle\_I for all individuals. 
Our method consistently outperforms MyStyle\_P and MyStyle\_I across all comparisons visually and numerically.
Detailed visual results can be found in Sec.~\ref{supp:vis_comp}, while additional numerical results are provided in Sec.~\ref{supp:num_comp}. 

\subsection{Additional Visual Results}
\label{supp:vis_comp}

In this section, we begin by presenting controlled image synthesis comparisons for all individuals. In the main paper, we have shown each attribute controlled image synthesis on different individuals. Here, we include image synthesis with all attributes controlled for each individual.
as shown in Figs.~\ref{fig_sup:sampling_bo}~through~\ref{fig_sup:sampling_ld} for Barack Obama, Michelle Obama, Oprah Winfrey, Taylor Swift, Emma Watson, and Leonardo DiCaprio, respectively.
Our method consistently achieves attribute-controlled image synthesis, in contrast to MyStyle\_I and MyStyle\_P, which exhibit significant inaccuracies in attribute controllability.

Next, we provide more visual comparison results for sampled image editing in Figs.~\ref{fig_sup:editing_sampled_bo}~through~\ref{fig_sup:editing_sampled_ld}. For each individual, we present the results of editing all the attributes. Our method ensures the preservation of identity and consistency of non-edited attributes, while editing the expression, yaw, pitch, or age of the image.

Lastly, we showcase more visual comparisons for real image editing in Fig.~\ref{fig_sup:editing_real}. Our method demonstrates improved attribute disentanglement compared to MyStyle\_P and MyStyle\_I. It produces results that effectively preserve the unchanged attributes and identity.

% ----------------------------------------------------------------------------
% ----------------------------------------------------------------------------
% ----------------------------------------------------------------------------

\subsection{Additional Numerical Results}
\label{supp:num_comp}

We first further numerically evaluate attribute controllability by by fixing one attribute and randomly sampling the other ones to generate images, using the same strategy introduced in the main paper. Here, we shown more comparisons on individuals, such as Barack Obama, Joe Biden, Michelle Obama, Oprah Winfrey, Taylor Swift, and Emma Watson, as shown in Table~\ref{sup_tab:syn_std_mean_1} and Table~\ref{sup_tab:syn_std_mean_2}. As seen, our approach consistently demonstrates the smallest standard deviation across all attributes for individuals.

Next, to ensure that the latent organization does not compromise the quality of the results, we evaluate our method against MyStyle using the ID metric~\cite{nitzan2022mystyle} and diversity score~\cite{ojha2021few} on more individuals, such as Barack Obama, Emma Watson, Joe Bide, Michelle Obama, Oprah Winfrey, and Taylor Swift. The comparison, presented in Table~\ref{tab_sup:syn_id_div}, demonstrates that our method produces results that are comparable to those of MyStyle.

We further conduct a numerical comparison of our real image editing results with MyStyle\_P and MyStyle\_I on Michelle Obama, Barack Obama, Joe Biden, Oprah Winfrey, Scarlett Johansson, Taylor Swift, and Emma Watson, as presented in Table~\ref{tab:edit_std}, Table~\ref{tab_sup:edit_std_1}, and Table~\ref{tab_sup:edit_std_2}. The results demonstrate the consistent superiority of our method over MyStyle\_P and MyStyle\_I across all metrics.

% ----------------------------------------------------------------------------
% ----------------------------------------------------------------------------
% ----------------------------------------------------------------------------
\begin{figure}[hbt]
\centering
\includegraphics[width=1.0\linewidth, scale=1.0, angle=-0]{supp_images/image_synthesis_sampling_yawpitchexp_V4_bo.pdf}
% \vspace{-0.2in}
\caption{We present a comparison of our synthesis results with those of MyStyle\_I and MyStyle\_P on Barack Obama.}
\vspace{-0.1in}
\label{fig_sup:sampling_bo}
\end{figure}

% ----------------------------------------------------------------------------
% \begin{figure}
% \centering
% \includegraphics[width=1.0\linewidth, scale=1.0, angle=-0]{supp_images/image_synthesis_sampling_yawpitchexp_V4_jb.pdf}
% % \vspace{-0.2in}
% \caption{We present a comparison of our synthesis results with those of MyStyle\_I and MyStyle\_P on Joe Biden.}
% \vspace{-0.1in}
% \label{fig_sup:sampling_jb}
% \end{figure}

% ----------------------------------------------------------------------------
\begin{figure}
\centering
\includegraphics[width=1.0\linewidth, scale=1.0, angle=-0]{supp_images/image_synthesis_sampling_yawpitchexp_V4_mo.pdf}
% \vspace{-0.2in}
\caption{We present a comparison of our synthesis results with those of MyStyle\_I and MyStyle\_P on Michelle Obama.}
\vspace{-0.1in}
\label{fig_sup:sampling_mo}
\end{figure}

% ----------------------------------------------------------------------------
\begin{figure}
\centering
\includegraphics[width=1.0\linewidth, scale=1.0, angle=-0]{supp_images/image_synthesis_sampling_yawpitchexp_V4_ow.pdf}
% \vspace{-0.2in}
\caption{We present a comparison of our synthesis results with those of MyStyle\_I and MyStyle\_P on Oprah Winfrey.}
\vspace{-0.1in}
\label{fig_sup:sampling_ow}
\end{figure}

% ----------------------------------------------------------------------------
% \begin{figure}
% \centering
% \includegraphics[width=1.0\linewidth, scale=1.0, angle=-0]{supp_images/image_synthesis_sampling_yawpitchexp_V4_sj.pdf}
% % \vspace{-0.2in}
% \caption{We present a comparison of our synthesis results with those of MyStyle\_I and MyStyle\_P on Scarlett Johansson.}
% \vspace{-0.1in}
% \label{fig_sup:sampling_sj}
% \end{figure}

% ----------------------------------------------------------------------------
\begin{figure}
\centering
\includegraphics[width=1.0\linewidth, scale=1.0, angle=-0]{supp_images/image_synthesis_sampling_yawpitchexp_V4_ts.pdf}
% \vspace{-0.2in}
\caption{We present a comparison of our synthesis results with those of MyStyle\_I and MyStyle\_P on Taylor Swift.}
\vspace{-0.1in}
\label{fig_sup:sampling_ts}
\end{figure}

% ----------------------------------------------------------------------------
\begin{figure}
\centering
\includegraphics[width=1.0\linewidth, scale=1.0, angle=-0]{supp_images/image_synthesis_sampling_yawpitchexpage_V4_ew.pdf}
% \vspace{-0.2in}
\caption{We present a comparison of our synthesis results with those of MyStyle\_I and MyStyle\_P on Emma Watson.}
\vspace{-0.1in}
\label{fig_sup:sampling_ew}
\end{figure}

% ----------------------------------------------------------------------------
\begin{figure}
\centering
\includegraphics[width=1.0\linewidth, scale=1.0, angle=-0]{supp_images/image_synthesis_sampling_yawpitchexpage_V4_ld.pdf}
% \vspace{-0.2in}
\caption{We present a comparison of our synthesis results with those of MyStyle\_I and MyStyle\_P on Leonardo DiCaprio.}
\vspace{-0.1in}
\label{fig_sup:sampling_ld}
\end{figure}

% ----------------------------------------------------------------------------
% ----------------------------------------------------------------------------
% ----------------------------------------------------------------------------

% ----------------------------------------------------------------------------
\begin{figure}
\centering
\includegraphics[width=\linewidth, scale=1.0, angle=-0]{supp_images/image_editing_sampled_v6_bo.pdf}
% \vspace{-0.2in}
\caption{We show our results for editing expression, yaw, and pitch angles for sampled images against MyStyle\_P and MyStyle\_I on Barack Obama. Our method maintains the identity and consistency of other attributes while making modifications to the expression, yaw, or pitch of the image.}
% \vspace{-0.1in}
\label{fig_sup:editing_sampled_bo}
\end{figure}

% ----------------------------------------------------------------------------
\begin{figure}
\centering
\includegraphics[width=\linewidth, scale=1.0, angle=-0]{supp_images/image_editing_sampled_v6_jb.pdf}
% \vspace{-0.2in}
\caption{We show our results for editing expression, yaw, and pitch angles for sampled images against MyStyle\_P and MyStyle\_I on Joe Biden. Our method maintains the identity and consistency of other attributes while making modifications to the expression, yaw, or pitch of the image.}
% \vspace{-0.1in}
\label{fig_sup:editing_sampled_jb}
\end{figure}

% ----------------------------------------------------------------------------
% \begin{figure}
% \centering
% \includegraphics[width=\linewidth, scale=1.0, angle=-0]{supp_images/image_editing_sampled_v6_mo.pdf}
% % \vspace{-0.2in}
% \caption{We show our results for editing expression, yaw, and pitch angles for sampled images against MyStyle\_P and MyStyle\_I on Michelle Obama. Our method maintains the identity and consistency of other attributes while making modifications to the expression, yaw, or pitch of the image.}
% % \vspace{-0.1in}
% \label{fig_sup:editing_sampled_mo}
% \end{figure}

% ----------------------------------------------------------------------------
\begin{figure}
\centering
\includegraphics[width=\linewidth, scale=1.0, angle=-0]{supp_images/image_editing_sampled_v6_sj.pdf}
% \vspace{-0.2in}
\caption{We show our results for editing expression, yaw, and pitch angles for sampled images against MyStyle\_P and MyStyle\_I on Scarlett Johansson. Our method maintains the identity and consistency of other attributes while making modifications to the expression, yaw, or pitch of the image.}
% \vspace{-0.1in}
\label{fig_sup:editing_sampled_sj}
\end{figure}

% ----------------------------------------------------------------------------
% \begin{figure}
% \centering
% \includegraphics[width=\linewidth, scale=1.0, angle=-0]{supp_images/image_editing_sampled_age_V7_em.pdf}
% % \vspace{-0.2in}
% \caption{We show our results for editing expression, yaw, and pitch angles for sampled images against MyStyle\_P and MyStyle\_I on Emma Watson. Our method maintains the identity and consistency of other attributes while making modifications to the expression, yaw, or pitch of the image.}
% % \vspace{-0.1in}
% \label{fig_sup:editing_sampled_ew}
% \end{figure}

% ----------------------------------------------------------------------------
\begin{figure}
\centering
\includegraphics[width=\linewidth, scale=1.0, angle=-0]{supp_images/image_editing_sampled_age_V6_ld.pdf}
% \vspace{-0.2in}
\caption{We show our results for editing expression, yaw, pitch, and age for sampled images against MyStyle\_P and MyStyle\_I on Leonardo DiCaprio. Our method maintains the identity and consistency of other attributes while making modifications to the expression, yaw, pitch, or age of the image.}
% \vspace{-0.1in}
\label{fig_sup:editing_sampled_ld}
\end{figure}

% ----------------------------------------------------------------------------
% ----------------------------------------------------------------------------
% ----------------------------------------------------------------------------

% ----------------------------------------------------------------------------
\begin{figure*}
\centering
\includegraphics[width=\linewidth, scale=1.0, angle=-0]{supp_images/image_editing_sup_V12.pdf}
% \vspace{-0.2in}
\caption{We show comparisons against both versions of MyStyle for semantic editing of real images. Input is the projected images into the latent space of MyStyle and our generators. Our method disentangles the attributes better than MyStyle\_P and MyStyle\_I, producing results that preserve the unchanged attributes and identity. InterFaceGAN~\cite{shen2020interfacegan} does not provide an edit direction for pitch, and thus we leave the corresponding area of MyStyle\_I with a cross.
}
% \vspace{-0.1in}
\label{fig_sup:editing_real}
\end{figure*}

% ----------------------------------------------------------------------------
% ----------------------------------------------------------------------------
% ----------------------------------------------------------------------------

% ----------------------------------------------------------------------------
% ----------------------------------------------------------------------------
% ----------------------------------------------------------------------------

% ----------------------------------------------------------------------------
% ----------------------------------------------------------------------------
\begin{table}[t] % not t or b or p
% \footnotesize
% \small
\caption{We numerically compare our controlled synthesis results against MyStyle\_P and MyStyle\_I. We generate 100 images for each fixed attribute value and report the standard deviation of the estimated attribute of interest over the generated images. Note that the attribute values (e.g., 0.25) are in the normalized coordinate $d_m$. The best results are shown in bold.}
%\vspace{-0.15in}
\centering
\begin{tabular}{ llccccc} 
% \begin{tabular*}{0.9\linewidth}{p{1.5cm} p{2.5cm} p{2.0cm} p{2.0cm} p{2.0cm} p{2.0cm}}
\hline
\hline
& & \multicolumn{5}{c}{Barack Obama} \\
\cmidrule(lr){3-7}
& & 0.0 & 0.25 & 0.5 & 0.75 & 1.0 \\
\hline
\multirow{3}{*}{Exp} & MyStyle\_P & 0.664 & 0.822 & 0.846 & 0.915 & 0.899 \\
& MyStyle\_I& 0.855 & 0.866 & 0.894 & 0.740 & 0.701 \\
& Ours & \textbf{0.241} & \textbf{0.575} & \textbf{0.582} & \textbf{0.457} & \textbf{0.003} \\
\hline
\multirow{3}{*}{Yaw} & MyStyle\_P & 4.072 & 6.349 & 4.168 & 5.258 & 5.289 \\
& MyStyle\_I & 5.858 & 5.530 & 5.249 & 3.364 & 5.360 \\
& Ours & \textbf{1.951} & \textbf{1.952} & \textbf{1.846} & \textbf{2.158} & \textbf{1.900} \\
\hline
\multirow{3}{*}{Pitch} & MyStyle\_P & 5.748 & 4.061 & 7.127 & 6.295 & 5.611 \\
& MyStyle\_I & - & - & - & - & - \\
& Ours & \textbf{1.670} & \textbf{2.198} & \textbf{2.851} & \textbf{3.413} & \textbf{3.336} \\
% \hline  
\end{tabular}
% ----------------------------------------------------------------------------
\centering
\begin{tabular}{ llccccc} 
% \begin{tabular*}{0.9\linewidth}{p{1.5cm} p{2.5cm} p{2.0cm} p{2.0cm} p{2.0cm} p{2.0cm}}
\hline
\hline
& & \multicolumn{5}{c}{Joe Biden} \\
\cmidrule(lr){3-7}
& & 0.0 & 0.25 & 0.5 & 0.75 & 1.0 \\
\hline
\multirow{3}{*}{Exp} & MyStyle\_P & 0.330 & 0.408 & 0.415 & 0.375 & 0.370 \\
& MyStyle\_I & 0.056 & 0.347 & 0.368 & 0.242 & 0.121 \\
& Ours & \textbf{0.031} & \textbf{0.216} & \textbf{0.329} & \textbf{221} & \textbf{0.013} \\
\hline
\multirow{3}{*}{Yaw} & MyStyle\_P & 6.725 & 6.411 & 5.071 & 9.103 & 7.652 \\
& MyStyle\_I & 5.578 & 3.777 & 3.474 & 4.832 & 6.687 \\
& Ours & \textbf{2.331} & \textbf{2.585} & \textbf{1.571} & \textbf{3.503} & \textbf{5.947} \\
\hline
\multirow{3}{*}{Pitch} & MyStyle\_P & 1.612 & 3.901 & 4.158 & 7.854 & 7.681 \\
& MyStyle\_I & - & - & - & - & - \\
& Ours & \textbf{4.061} & \textbf{3.669} & \textbf{1.431} & \textbf{2.464} & \textbf{2.117} \\
% \hline  
\end{tabular}
% ----------------------------------------------------------------------------
\centering
\begin{tabular}{ llccccc} 
% \begin{tabular*}{0.9\linewidth}{p{1.5cm} p{2.5cm} p{2.0cm} p{2.0cm} p{2.0cm} p{2.0cm}}
\hline
\hline
& & \multicolumn{5}{c}{Michelle Obama} \\
\cmidrule(lr){3-7}
& & 0.0 & 0.25 & 0.5 & 0.75 & 1.0 \\
\hline
\multirow{3}{*}{Exp} & MyStyle\_P & 0.478 & 0.601 & 0.828 & 0.612 & 0.655 \\
& MyStyle\_I& 0.872 & 0.798 & 0.521 & 0.361 & 0.001 \\
& Ours & \textbf{0.169} & \textbf{0.378} & \textbf{0.217} & \textbf{0.038} & \textbf{0.000} \\
\hline
\multirow{3}{*}{Yaw} & MyStyle\_P & 3.239 & 4.464 & 2.757 & 5.195 & 4.835 \\
& MyStyle\_I & 4.473 & 2.920 & 3.692 & 4.077 & 4.523 \\
& Ours & \textbf{1.197} & \textbf{1.581} & \textbf{1.796} & \textbf{1.717} & \textbf{1.488} \\
\hline
\multirow{3}{*}{Pitch} & MyStyle\_P & 3.902 & 4.673 & 4.661 & 3.547 & 3.823 \\
& MyStyle\_I & - & - & - & - & - \\
& Ours & \textbf{2.426} & \textbf{2.264} & \textbf{1.699} & \textbf{1.823} & \textbf{1.687} \\
% \hline  
\end{tabular}
% ----------------------------------------------------------------------------
\centering
\begin{tabular}{ llccccc} 
% \begin{tabular*}{0.9\linewidth}{p{1.5cm} p{2.5cm} p{2.0cm} p{2.0cm} p{2.0cm} p{2.0cm}}
\hline
\hline
& & \multicolumn{5}{c}{Oprah Winfrey} \\
\cmidrule(lr){3-7}
& & 0.0 & 0.25 & 0.5 & 0.75 & 1.0 \\
\hline
\multirow{3}{*}{Exp} & MyStyle\_P & 0.425 & 0.509 & 0.039 & 0.0024 & 0.006 \\
& MyStyle\_I& 0.067 & 0.371 & 0.003 & 0.009 & 0.002 \\
& Ours & \textbf{0.048} & \textbf{0.293} & \textbf{0.002} & \textbf{0.003} & \textbf{0.001} \\
\hline
\multirow{3}{*}{Yaw} & MyStyle\_P & 5.905 & 4.397 & 7.275 & 3.844 & 6.130 \\
& MyStyle\_I & 3.069 & 3.180 & 2.136 & 2.605 & 3.686 \\
& Ours & \textbf{1.333} & \textbf{2.704} & \textbf{1.649} & \textbf{1.532} & \textbf{1.119} \\
\hline
\multirow{3}{*}{Pitch} & MyStyle\_P & 4.551 & 4.470 & 3.765 & 3.788 & 4.181 \\
& MyStyle\_I & - & - & - & - & - \\
& Ours & \textbf{1.509} & \textbf{2.520} & \textbf{1.622} & \textbf{1.729} & \textbf{1.797} \\
\hline  
\end{tabular}

\label{sup_tab:syn_std_mean_1}
%\vspace{-0.2in}
\end{table}

% ----------------------------------------------------------------------------
% ----------------------------------------------------------------------------
\begin{table}[t] % not t or b or p
% \footnotesize
% \small
\caption{We numerically compare our controlled synthesis results against MyStyle\_P and MyStyle\_I. We generate 100 images for each fixed attribute value and report the standard deviation of the estimated attribute of interest over the generated images. Note that the attribute values (e.g., 0.25) are in the normalized coordinate $d_m$. The best results are shown in bold.}
%\vspace{-0.15in}
\centering
\begin{tabular}{ llccccc} 
% \begin{tabular*}{0.9\linewidth}{p{1.5cm} p{2.5cm} p{2.0cm} p{2.0cm} p{2.0cm} p{2.0cm}}
\hline
\hline
& & \multicolumn{5}{c}{Taylor Swift} \\
\cmidrule(lr){3-7}
& & 0.0 & 0.25 & 0.5 & 0.75 & 1.0 \\
\hline
\multirow{3}{*}{Exp} & MyStyle\_P & 0.673 & 0.612 & 0.582 & 0.611 & 300 \\
& MyStyle\_I& 0.361 & 0.602 & 0.355 & 0.690 & 0.677 \\
& Ours & \textbf{0.296} & \textbf{0.415} & \textbf{0.284} & \textbf{0.405} & \textbf{0.414} \\
\hline
\multirow{3}{*}{Yaw} & MyStyle\_P & 5.287 & 4.799 & 5.436 & 6.135 & 6.131 \\
& MyStyle\_I & 4.629 & 4.886 & 3.414 & 6.090 & 4.444 \\
& Ours & \textbf{1.618} & \textbf{2.187} & \textbf{2.843} & \textbf{2.443} & \textbf{1.657} \\
\hline
\multirow{3}{*}{Pitch} & MyStyle\_P & 5.012 & 5.005 & 2.566 & 3.089 & 4.156 \\
& MyStyle\_I & - & - & - & - & - \\
& Ours & \textbf{3.513} & \textbf{2.189} & \textbf{2.304} & \textbf{2.395} & \textbf{2.261} \\
% \hline  
\end{tabular}
% ----------------------------------------------------------------------------
\centering
\begin{tabular}{ llccccc} 
% \begin{tabular*}{0.9\linewidth}{p{1.5cm} p{2.5cm} p{2.0cm} p{2.0cm} p{2.0cm} p{2.0cm}}
\hline
\hline
& & \multicolumn{5}{c}{Emma Watson}\\
\cmidrule(lr){3-7}
& & 0.0 & 0.25 & 0.5 & 0.75 & 1.0 \\
\hline
\multirow{3}{*}{Exp} & MyStyle\_P & 0.899 & 0.738 & 0.883 & 0.786 & 0.482 \\
& MyStyle\_I & 0.273 & 0.0.583 & 0.777 & 0.313 & 0.002 \\
& Ours & \textbf{0.005} & \textbf{0.004} & \textbf{0.531} & \textbf{0.213} & \textbf{0.001} \\
\hline
\multirow{3}{*}{Yaw} & MyStyle\_P & 4.353 & 5.834 & 5.156 & 4.268 & 3.948 \\
& MyStyle\_I & 3.277 & 3.146 & 1.997 & 3.133 & 3.080 \\
& Ours & \textbf{1.745} & \textbf{2.495} & \textbf{1.431} & \textbf{2.339} & \textbf{2.127} \\
\hline
\multirow{3}{*}{Pitch} & MyStyle\_P & 6.645 & 6.094 & 4.485 & 2.988 & 1.808 \\
& MyStyle\_I & - & - & - & - & -\\
& Ours & \textbf{4.887} & \textbf{2.714} & \textbf{1.758} & \textbf{2.374} & \textbf{1.426} \\
\hline
\multirow{3}{*}{Age} & MyStyle\_P & 2.760 & 2.016 & 0.899 & 1.041 & 1.062 \\
& MyStyle\_I & 3.775 & 2.502 & 0.873 & 1.171 & 1.920 \\
& Ours & \textbf{1.734} & \textbf{1.405} & \textbf{0.607} & \textbf{1.001} & \textbf{0.910} \\
\hline  
\end{tabular}
\label{sup_tab:syn_std_mean_2}
%\vspace{-0.2in}
\end{table}

% ----------------------------------------------------------------------------
% ----------------------------------------------------------------------------
% ----------------------------------------------------------------------------

% ----------------------------------------------------------------------------
% ----------------------------------------------------------------------------
\begin{table}[t] % not t or b or p
% \footnotesize
% \small
\caption{We compare our results against MyStyle in terms of the ID metric~\cite{nitzan2022mystyle} and diversity score~\cite{ojha2021few}. Higher numbers are better. Our method produces similar results compared to MyStyles, which demonstrates that controllability does not hurt our system.}
\centering
\begin{tabular}{ >{\arraybackslash}m{0.7in} >{\arraybackslash}m{0.5in} >{\centering\arraybackslash}m{0.75in} >{\centering\arraybackslash}m{0.75in} }
% \begin{tabular}{ llc|c} 
% \begin{tabular*}{0.9\linewidth}{p{1.5cm} p{2.5cm} p{2.0cm} p{2.0cm} p{2.0cm} p{2.0cm}}
\hline
\hline
& & \multicolumn{1}{c}{ID $\uparrow$ } & \multicolumn{1}{c}{Diversity $\uparrow$ }\\
% \cmidrule(lr){2-3}
% \cmidrule(lr){4-5}
\hline
\multirow{2}{*}{Barack Obama} & MyStyle & 0.787$\pm$0.053 & 0.393$\pm$0.070 \\
& Ours & 0.796$\pm$0.050 & 0.411$\pm$0.026 \\
\hline
\multirow{2}{*}{Emma Watson} & MyStyle & 0.734$\pm$0.090 & 0.453$\pm$0.023 \\
& Ours & 0.742$\pm$0.061 & 0.449$\pm$0.018 \\
\hline
\multirow{2}{*}{Joe Biden} & MyStyle & 0.759$\pm$0.004 & 0.397$\pm$0.023 \\
& Ours & 0.761$\pm$0.001 & 0.402$\pm$0.044 \\
\hline
\multirow{2}{*}{Michelle Obama} & MyStyle & 0.752$\pm$0.003  & 0.391$\pm$0.039 \\
& Ours & 0.757$\pm$0.004 & 0.389$\pm$0.024\\
\hline
\multirow{2}{*}{Oprah Winfrey} & MyStyle & 0.807$\pm$0.053 & 0.380$\pm$0.038 \\
& Ours & 0.821$\pm$0.058 & 0.380$\pm$0.057 \\
\hline
\multirow{2}{*}{Taylor Swift} & MyStyle & 0.775$\pm$0.065 & 0.393$\pm$0.049 \\
& Ours & 0.774$\pm$0.067 & 0.403$\pm$0.019 \\

\hline  
\end{tabular}
\label{tab_sup:syn_id_div}
\end{table}

% ----------------------------------------------------------------------------
% ----------------------------------------------------------------------------
% ----------------------------------------------------------------------------

% -----------------------moved--from--main------------------------------------
% ----------------------------------------------------------------------------
\begin{table}[htb] % not t or b or p
% \footnotesize
% \small
\caption{We compare our editing results against MyStyle\_I and MyStyle\_P in terms of the mean standard deviation (STD) of the edited attribute to show editing consistency (marked with $*$), and of fixed attributes to demonstrate attribute disentanglement. We additionally report the ID metric to evaluate identity preservation ability. The best results are shown in bold.}
\vspace{-0.15in}
\centering
\begin{tabular}{p{0.03\textwidth}>
{}p{0.07\textwidth}>
{\centering}p{0.05\textwidth}>
{\centering}p{0.05\textwidth}>
{\centering}p{0.05\textwidth}>
{\centering\arraybackslash}p{0.1\textwidth}}
% \begin{tabular*}{0.9\linewidth}{p{1.5cm} p{2.5cm} p{2.0cm} p{2.0cm} p{2.0cm} p{2.0cm}}
\hline
\hline
& & \multicolumn{4}{c}{Michelle Obama} \\
\cmidrule(lr){1-2}
\cmidrule(lr){3-6}
& & Exp$^{*}$ & Yaw & Pitch & ID $\uparrow$\\
\cmidrule(lr){3-3}
\cmidrule(lr){4-5}
\cmidrule(lr){6-6}
\multirow{3}{*}{Exp} & MyStyle\_P  & 0.547 & 0.716 & 4.436 & 0.786$\pm$0.057\\
& MyStyle\_I  & 0.445 & 1.069 & 0.715 & 0.757$\pm$0.065 \\
& Ours & \textbf{0.306} & \textbf{0.576} & \textbf{0.596} & \textbf{0.794$\pm$0.034} \\

\hline
& & Yaw$^{*}$ & Exp & Pitch & ID $\uparrow$\\
\cmidrule(lr){3-3}
\cmidrule(lr){4-5}
\cmidrule(lr){6-6}
\multirow{3}{*}{Yaw} & MyStyle\_P  & 2.773 & 0.477 & 2.419 & 0.780$\pm$0.053\\
& MyStyle\_I  & 4.424 & 0.510 & 2.181 & 0.715$\pm$0.110\\
& Ours  & \textbf{0.876} & \textbf{0.298} & \textbf{1.137} & \textbf{0.792$\pm$0.047} \\

\hline
& & Pitch$^{*}$ & Exp & Yaw & ID $\uparrow$\\
\cmidrule(lr){3-3}
\cmidrule(lr){4-5}
\cmidrule(lr){6-6}
\multirow{3}{*}{Pitch} & MyStyle\_P  & 6.306 & 0.463 & 2.242 & 0.727$\pm$0.047\\
& MyStyle\_I & - & - & - & -\\
& Ours  & \textbf{2.045} & \textbf{0.231} & \textbf{1.311} & \textbf{0.731$\pm$0.110} \\
\hline  
\end{tabular}

\label{tab:edit_std}
\vspace{-0.15in}
\end{table}

% ----------------------------------------------------------------------------
% ----------------------------------------------------------------------------
\begin{table}[t] % not t or b or p
% \footnotesize
% \small
\caption{We compare our editing results against MyStyle\_I and MyStyle\_P in terms of the mean standard deviation (STD) of edited attribute to show editing consistency (marked with $*$), and of fixed attributes to demonstrate attribute disentanglement. We additionally report the ID metric to evaluate identity preservation ability. The best results are shown in bold.}
%\vspace{-0.00in}
\centering
\begin{tabular}{p{0.03\textwidth}>
{}p{0.07\textwidth}>
{\centering}p{0.05\textwidth}>
{\centering}p{0.05\textwidth}>
{\centering}p{0.05\textwidth}>
{\centering\arraybackslash}p{0.1\textwidth}}
% \begin{tabular*}{0.9\linewidth}{p{1.5cm} p{2.5cm} p{2.0cm} p{2.0cm} p{2.0cm} p{2.0cm}}
\hline
\hline
& & \multicolumn{4}{c}{Barack Obama} \\
\cmidrule(lr){1-2}
\cmidrule(lr){3-6}
& & Exp$^{*}$ & Yaw & Pitch & ID $\uparrow$\\
\cmidrule(lr){3-3}
\cmidrule(lr){4-5}
\cmidrule(lr){6-6}
\multirow{3}{*}{Exp} & MyStyle\_P  & 0.156 & 5.502 & 2.265 & 0.700$\pm$0.087\\
& MyStyle\_I  & 0.261 & 1.751 & 1.808 & 0.703$\pm$0.086\\
& Ours & \textbf{0.107} & \textbf{0.533} & \textbf{0.804} & \textbf{0.742$\pm$0.079} \\

\hline
& & Yaw$^{*}$ & Exp & Pitch & ID $\uparrow$\\
\cmidrule(lr){3-3}
\cmidrule(lr){4-5}
\cmidrule(lr){6-6}
\multirow{3}{*}{Yaw} & MyStyle\_P  & 4.310 & 0.054 & 5.727 & 0.689$\pm$0.085\\
& MyStyle\_I  & 3.117 & 0.043 & 3.770 & 0.687$\pm$0.087\\
& Ours  & \textbf{1.524} & \textbf{0.028} & \textbf{2.349} & \textbf{0.709$\pm$0.083} \\

\hline
& & Pitch$^{*}$ & Exp & Yaw & ID $\uparrow$\\
\cmidrule(lr){3-3}
\cmidrule(lr){4-5}
\cmidrule(lr){6-6}
\multirow{3}{*}{Pitch} & MyStyle\_P  & 5.131 & 0.031 & 6.285 & 0.692$\pm$0.087\\
& MyStyle\_I & - & - & - & -\\
& Ours  & \textbf{2.990} & \textbf{0.026} & \textbf{1.055} & \textbf{0.709$\pm$0.084} \\
% \hline  
\end{tabular}
% ----------------------------------------------------------------------------
\centering
\begin{tabular}{p{0.03\textwidth}>
{}p{0.07\textwidth}>
{\centering}p{0.05\textwidth}>
{\centering}p{0.05\textwidth}>
{\centering}p{0.05\textwidth}>
{\centering\arraybackslash}p{0.1\textwidth}}
% \begin{tabular*}{0.9\linewidth}{p{1.5cm} p{2.5cm} p{2.0cm} p{2.0cm} p{2.0cm} p{2.0cm} p{2.0cm}}
\hline
\hline
& & \multicolumn{4}{c}{Joe Biden} \\
\cmidrule(lr){1-2}
\cmidrule(lr){3-6}
& & Exp$^{*}$ & Yaw & Pitch & ID $\uparrow$\\
\cmidrule(lr){3-3}
\cmidrule(lr){4-5}
\cmidrule(lr){6-6}
\multirow{3}{*}{Exp} & MyStyle\_P  & 0.776 & 1.809 & 5.619 & 0.654$\pm$0.091\\
& MyStyle\_I  & 0.446 & 1.707 & 1.054 & 0.693$\pm$0.072\\
& Ours & \textbf{0.332} & \textbf{1.095} & \textbf{1.254} & \textbf{0.703$\pm$0.076} \\
\hline
& & Yaw$^{*}$ & Exp & Pitch & ID $\uparrow$\\
\cmidrule(lr){3-3}
\cmidrule(lr){4-5}
\cmidrule(lr){6-6}
\multirow{3}{*}{Yaw} & MyStyle\_P  & 10.42 & 0.739 & 10.50 & 0.666$\pm$0.084\\
& MyStyle\_I   & 9.190 & 0.789 & 2.341 & 0.676$\pm$0.077\\
& Ours  & \textbf{3.425} & \textbf{0.625} & \textbf{2.205} & \textbf{0.705$\pm$0.072} \\

\hline
& & Pitch$^{*}$ & Exp & Yaw & ID $\uparrow$\\
\cmidrule(lr){3-3}
\cmidrule(lr){4-5}
\cmidrule(lr){6-6}
\multirow{3}{*}{Pitch} & MyStyle\_P   & 9.262 & 0.786 & 18.06 & 0.637$\pm$0.111\\
& MyStyle\_I & - & - & - & - \\
& Ours  & \textbf{3.958} & \textbf{0.603} & \textbf{2.656} & \textbf{0.693$\pm$0.080} \\
% \hline  
\end{tabular}
% ----------------------------------------------------------------------------
\centering
\begin{tabular}{p{0.03\textwidth}>
{}p{0.07\textwidth}>
{\centering}p{0.05\textwidth}>
{\centering}p{0.05\textwidth}>
{\centering}p{0.05\textwidth}>
{\centering\arraybackslash}p{0.1\textwidth}}
% \begin{tabular*}{0.9\linewidth}{p{1.5cm} p{2.5cm} p{2.0cm} p{2.0cm} p{2.0cm} p{2.0cm} p{2.0cm}}
\hline
\hline
& & \multicolumn{4}{c}{Oprah Winfrey} \\
\cmidrule(lr){1-2}
\cmidrule(lr){3-6}
& & Exp$^{*}$ & Yaw & Pitch & ID $\uparrow$\\
\cmidrule(lr){3-3}
\cmidrule(lr){4-5}
\cmidrule(lr){6-6}
\multirow{3}{*}{Exp} & MyStyle\_P  & 0.303 & 4.358 & 3.335 & 0.685$\pm$0.100\\
& MyStyle\_I  & 0.140 & 1.738 & 1.523 & 0.690$\pm$0.092\\
& Ours & \textbf{0.116} & \textbf{0.531} & \textbf{0.401} & \textbf{0.712$\pm$0.088} \\
\hline
& & Yaw$^{*}$ & Exp & Pitch & ID $\uparrow$\\
\cmidrule(lr){3-3}
\cmidrule(lr){4-5}
\cmidrule(lr){6-6}
\multirow{3}{*}{Yaw} & MyStyle\_P & 6.338 & 0.052 & 5.284 & 0.695$\pm$0.075\\
& MyStyle\_I  & 5.242 & 0.039 & 3.250 & 0.698$\pm$0.074\\
& Ours  & \textbf{2.330} & \textbf{0.027} & \textbf{2.425} & \textbf{0.702$\pm$0.075} \\

\hline
& & Pitch$^{*}$ & Exp & Yaw & ID $\uparrow$\\
\cmidrule(lr){3-3}
\cmidrule(lr){4-5}
\cmidrule(lr){6-6}
\multirow{3}{*}{Pitch} & MyStyle\_P  & 4.949 & 0.053 & 3.423 & 0.657$\pm$0.104\\
& MyStyle\_I & - & - & - & - \\
& Ours  & \textbf{2.001} & \textbf{0.031} & \textbf{1.445} & \textbf{0.698$\pm$0.070} \\

\hline  
\end{tabular}

\label{tab_sup:edit_std_1}
%\vspace{-0.2in}
\end{table}

% ----------------------------------------------------------------------------
% ----------------------------------------------------------------------------
% ----------------------------------------------------------------------------
\begin{table}[htb] % not t or b or p
% \footnotesize
% \small
\caption{We compare our editing results against MyStyle\_I and MyStyle\_P in terms of the mean standard deviation (STD) of edited attribute to show editing consistency (marked with $*$), and of fixed attributes to demonstrate attribute disentanglement. We additionally report the ID metric to evaluate identity preservation ability. The best results are shown in bold.}
%\vspace{-0.00in}
\centering
\begin{tabular}{p{0.03\textwidth}>
{}p{0.07\textwidth}>
{\centering}p{0.05\textwidth}>
{\centering}p{0.05\textwidth}>
{\centering}p{0.05\textwidth}>
{\centering\arraybackslash}p{0.1\textwidth}}
% \begin{tabular*}{0.9\linewidth}{p{1.5cm} p{2.5cm} p{2.0cm} p{2.0cm} p{2.0cm} p{2.0cm}}
\hline
\hline
& & \multicolumn{4}{c}{Scarlett Johansson} \\
\cmidrule(lr){1-2}
\cmidrule(lr){3-6}
& & Exp$^{*}$ & Yaw & Pitch & ID $\uparrow$\\
\cmidrule(lr){3-3}
\cmidrule(lr){4-5}
\cmidrule(lr){6-6}
\multirow{3}{*}{Exp} & MyStyle\_P  & 0.866 & 2.578 & 3.942 & 0.666$\pm$0.075\\
& MyStyle\_I  & 0.328 & 1.131 & 0.577 & 0.660$\pm$0.090\\
& Ours & \textbf{0.270} & \textbf{0.607} & \textbf{0.510} & \textbf{0.675$\pm$0.074} \\
\hline
& & Yaw$^{*}$ & Exp & Pitch & ID $\uparrow$\\
\cmidrule(lr){3-3}
\cmidrule(lr){4-5}
\cmidrule(lr){6-6}
\multirow{3}{*}{Yaw} & MyStyle\_P & 9.216 & 0.869 & 1.671 & 0.686 $\pm$0.078\\
& MyStyle\_I   & 4.655 & 0.859 & 2.270 & 0.645$\pm$0.082\\
& Ours  & \textbf{2.349} & \textbf{0.774} & \textbf{1.669} & \textbf{0.707$\pm$0.069} \\

\hline
& & Pitch$^{*}$ & Exp & Yaw & ID $\uparrow$\\
\cmidrule(lr){3-3}
\cmidrule(lr){4-5}
\cmidrule(lr){6-6}
\multirow{3}{*}{Pitch} & MyStyle\_P   & 5.639 & 0.924 & 5.755 & 0.667$\pm$0.077\\
& MyStyle\_I & - & - & - & - \\
& Ours  & \textbf{4.130} & \textbf{0.793} & \textbf{1.316} & \textbf{0.684$\pm$0.076} \\
% \hline  
\end{tabular}
% ----------------------------------------------------------------------------
\centering
\begin{tabular}{p{0.03\textwidth}>
{}p{0.07\textwidth}>
{\centering}p{0.05\textwidth}>
{\centering}p{0.05\textwidth}>
{\centering}p{0.05\textwidth}>
{\centering\arraybackslash}p{0.1\textwidth}}
% \begin{tabular*}{0.9\linewidth}{p{1.5cm} p{2.5cm} p{2.0cm} p{2.0cm} p{2.0cm} p{2.0cm} p{2.0cm}}
\hline
\hline
& & \multicolumn{4}{c}{Taylor Swift} \\
\cmidrule(lr){1-2}
\cmidrule(lr){3-6}
& & Exp$^{*}$ & Yaw & Pitch & ID $\uparrow$\\
\cmidrule(lr){3-3}
\cmidrule(lr){4-5}
\cmidrule(lr){6-6}
\multirow{3}{*}{Exp} & MyStyle\_P  & 0.783 & 3.421 & 3.933 & 0.698$\pm$0.077\\
& MyStyle\_I  & 0.314 & 2.444 & 1.237 & 0.683$\pm$0.079\\
& Ours & \textbf{0.230} & \textbf{1.532} & \textbf{0.783} & \textbf{0.713$\pm$0.077} \\
\hline
& & Yaw$^{*}$ & Exp & Pitch & ID $\uparrow$\\
\cmidrule(lr){3-3}
\cmidrule(lr){4-5}
\cmidrule(lr){6-6}
\multirow{3}{*}{Yaw} & MyStyle\_P  & 7.343 & 0.783 & 3.210 & 0.688$\pm$0.087\\
& MyStyle\_I   & 3.598 & 0.389 & 2.333 & 0.700$\pm$0.074\\
& Ours  & \textbf{1.925} & \textbf{0.241} & \textbf{1.982} & \textbf{0.720$\pm$0.069} \\

\hline
& & Pitch$^{*}$ & Exp & Yaw & ID $\uparrow$\\
\cmidrule(lr){3-3}
\cmidrule(lr){4-5}
\cmidrule(lr){6-6}
\multirow{3}{*}{Pitch} & MyStyle\_P   & 4.189 & 0.102 & 5.283 & 0.703$\pm$0.078\\
& MyStyle\_I & - & - & - & - \\
& Ours  & \textbf{2.374} & \textbf{0.041} & \textbf{2.338} & \textbf{0.721$\pm$0.079} \\
% \hline  
\end{tabular}
% ----------------------------------------------------------------------------
\centering
\begin{tabular}{p{0.03\textwidth}>
{}p{0.07\textwidth}>
{\centering}p{0.035\textwidth}>
{\centering}p{0.035\textwidth}>
{\centering}p{0.035\textwidth}>
{\centering}p{0.035\textwidth}>
{\centering\arraybackslash}p{0.1\textwidth}}
% \begin{tabular*}{0.9\linewidth}{p{1.5cm} p{2.5cm} p{2.0cm} p{2.0cm} p{2.0cm} p{2.0cm} p{2.0cm}}
\hline
\hline
& & \multicolumn{5}{c}{Emma Watson} \\
\cmidrule(lr){1-2}
\cmidrule(lr){3-7}
& & Exp$^{*}$ & Yaw & Pitch & Age & ID $\uparrow$\\
\cmidrule(lr){3-3}
\cmidrule(lr){4-6}
\cmidrule(lr){7-7}
\multirow{3}{*}{Exp} & MyStyle\_P  & 0.821  & 3.892 & 2.721 & 4.021 & 0.698$\pm$0.113\\
& MyStyle\_I   & 0.482  & 1.732 & 2.034 & 3.248 & 0.710$\pm$0.096\\
& Ours & \textbf{0.240} & \textbf{1.330} & \textbf{1.218} & \textbf{2.017} & \textbf{0.748$\pm$0.094} \\
\hline
& & Yaw$^{*}$ & Exp & Pitch & Age & ID $\uparrow$\\
\cmidrule(lr){3-3}
\cmidrule(lr){4-6}
\cmidrule(lr){7-7}
\multirow{3}{*}{Yaw} & MyStyle\_P   & 5.478  & 0.432 & 3.258 & 3.483 & 0.728$\pm$0.090\\
& MyStyle\_I  & 4.130  & 0.384& 2.832 & 3.003 & 0.713$\pm$0.094\\
& Ours  & \textbf{2.783} & \textbf{0.104} & \textbf{2.203} & \textbf{2.438} & \textbf{0.733$\pm$0.092} \\

\hline
& & Pitch$^{*}$ & Exp & Yaw & Age & ID $\uparrow$\\
\cmidrule(lr){3-3}
\cmidrule(lr){4-6}
\cmidrule(lr){7-7}
\multirow{3}{*}{Pitch} & MyStyle\_P   & 4.389  & 0.492 & 3.189 & 3.899 & 0.728$\pm$0.096\\
& MyStyle\_I & - & - & - & - & -\\
& Ours  & \textbf{3.294} & \textbf{0.085} & \textbf{1.839} & \textbf{2.893} & \textbf{0.746$\pm$0.094} \\

\hline
& & Age$^{*}$ & Exp & Yaw & Pitch & ID $\uparrow$\\
\cmidrule(lr){3-3}
\cmidrule(lr){4-6}
\cmidrule(lr){7-7}
\multirow{3}{*}{Age} & MyStyle\_P   & 4.883  & 0.432 & 3.543 & 2.983 & 0.717$\pm$0.086\\
& MyStyle\_I  & 4.238  & 0.233 & 2.899 & 2.339 & 0.725$\pm$0.114\\
& Ours  & \textbf{2.938} & \textbf{0.183} & \textbf{1.032} & \textbf{1.384} & \textbf{0.742$\pm$0.082} \\
\hline  
\end{tabular}

\label{tab_sup:edit_std_2}
%\vspace{-0.2in}
\end{table}
